# Supplementary material for: The Quantum Pendulum of Turbulent Flow: Decaying turbulence as a thermal state of an integrable system
Source: arXiv:2607.05745 source file (2026-11-16)
Supplement: Supplementary file 1 [file Supplement_labels.tex]

% Labels regenerated from Supplement.aux (anchor and file fields blank).
% Revision (ab) of 2026-11-16: regenerated; no number changed.
\makeatletter
\newlabel{sec:S-intro-details}{{S1}{4}{The Introduction: details}{}{}}
\newlabel{rem:intro-positivity}{{S1.1}{6}{}{}{}}
\newlabel{sec:S-mle}{{S2}{10}{The momentum-loop equation: details}{}{}}
\newlabel{eq:physical-ns-vector}{{S2.1}{10}{The momentum-loop equation: details}{}{}}
\newlabel{sec:S-mle-proofs}{{S2.1}{11}{The operator identity and the calculus of jumps}{}{}}
\newlabel{eq:qsp-pexp}{{S2.2}{11}{The operator identity}{}{}}
\newlabel{eq:qsp-transport}{{S2.3}{11}{The operator identity}{}{}}
\newlabel{sec:S-qsp-examples}{{S3}{13}{The Quantum Statistical Principle: the correspondence and the examples}{}{}}
\newlabel{sec:S-qsp-correspondence}{{S3.1}{13}{Classical statistics and quantum mechanics}{}{}}
\newlabel{sec:qsp-gibbs}{{S3.2}{13}{The Gibbs distribution}{}{}}
\newlabel{eq:qsp-thermal}{{S3.1}{13}{The Gibbs distribution}{}{}}
\newlabel{eq:qsp-perimeter}{{S3.2}{14}{The Gibbs distribution}{}{}}
\newlabel{eq:qsp-white}{{S3.3}{14}{The Gibbs distribution}{}{}}
\newlabel{eq:qsp-gibbs-field}{{S3.4}{14}{The operator form}{}{}}
\newlabel{eq:qsp-gibbs-displacement}{{S3.5}{14}{The operator form}{}{}}
\newlabel{eq:qsp-gibbs-W}{{S3.6}{14}{Proper time}{}{}}
\newlabel{sec:qsp-rotation}{{S3.3}{15}{The uniform rotation}{}{}}
\newlabel{eq:qsp-rotation}{{S3.7}{15}{The uniform rotation}{}{}}
\newlabel{eq:qsp-rotation-loop}{{S3.8}{15}{The uniform rotation}{}{}}
\newlabel{eq:qsp-rotation-correlator}{{S3.9}{15}{The uniform rotation}{}{}}
\newlabel{eq:qsp-rotation-action}{{S3.10}{15}{Quantization}{}{}}
\newlabel{eq:qsp-rotation-commutator}{{S3.11}{15}{Quantization}{}{}}
\newlabel{eq:qsp-oscillator}{{S3.12}{15}{Quantization}{}{}}
\newlabel{eq:qsp-holonomy}{{S3.13}{16}{The exact trace}{}{}}
\newlabel{eq:qsp-ordered}{{S3.14}{16}{The state}{}{}}
\newlabel{eq:qsp-vorticity}{{S3.15}{16}{Vorticity as a commutator}{}{}}
\newlabel{sec:qsp-rotating}{{S3.4}{17}{The rotating fluid in thermal equilibrium}{}{}}
\newlabel{eq:qsp-rotating}{{S3.16}{17}{The rotating fluid in thermal equilibrium}{}{}}
\newlabel{eq:qsp-rotating-P}{{S3.17}{17}{The rotating fluid in thermal equilibrium}{}{}}
\newlabel{sec:S-qsp-euler}{{S3.5}{17}{The Euler ensemble in the language of the principle}{}{}}
\newlabel{sec:qsp-stochasticity}{{S3.6}{18}{A representation suited to spontaneous stochasticity}{}{}}
\newlabel{sec:S-qsp}{{S4}{19}{The Quantum Statistical Principle: details}{}{}}
\newlabel{eq:S-qsp-area}{{S4.1}{19}{The area tensor of a polygon}{}{}}
\newlabel{eq:S-qsp-area-identities}{{S4.2}{19}{The area tensor of a polygon}{}{}}
\newlabel{eq:S-qsp-cot}{{S4.3}{19}{Antiperiodic modes}{}{}}
\newlabel{eq:S-qsp-modes}{{S4.4}{19}{Antiperiodic modes}{}{}}
\newlabel{eq:S-qsp-halfinteger}{{S4.5}{19}{Antiperiodic modes}{}{}}
\newlabel{eq:S-qsp-bch}{{S4.6}{20}{The ordered product}{}{}}
\newlabel{sec:bv-sphere}{{S5}{21}{Jumps, the sphere, and the spherical-sector postulate}{}{}}
\newlabel{eq:spherical-telescoping}{{S5.1}{22}{Spherical confinement}{}{}}
\newlabel{eq:diffusive-stationary-geometry}{{S5.2}{22}{Spherical confinement}{}{}}
\newlabel{sec:S-bv}{{S6}{22}{The calculus of jumps}{}{}}
\newlabel{eq:variation-divergence}{{S6.1}{23}{The calculus of jumps}{}{}}
\newlabel{sec:S-contact}{{S7}{23}{The second area derivative: derivation}{}{}}
\newlabel{eq:ct-tangent}{{S7.1}{23}{The second area derivative: derivation}{}{}}
\newlabel{eq:ct-area-operator}{{S7.2}{23}{The second area derivative: derivation}{}{}}
\newlabel{eq:ct-chain}{{S7.3}{23}{The second area derivative: derivation}{}{}}
\newlabel{eq:ct-product}{{S7.4}{24}{The second area derivative: derivation}{}{}}
\newlabel{eq:ct-product-fixed}{{S7.5}{24}{The second area derivative: derivation}{}{}}
\newlabel{eq:ct-kick}{{S7.6}{24}{The second area derivative: derivation}{}{}}
\newlabel{sec:S-ct-polygon}{{S7.1}{25}{The polygon: the pair weight and the normalization}{}{}}
\newlabel{eq:ct-polygon}{{S7.7}{25}{The polygon: the pair weight and the normalization}{}{}}
\newlabel{eq:ct-normalized}{{S7.8}{25}{The normalization}{}{}}
\newlabel{sec:S-contact-main}{{S7.2}{25}{The rule at the mark, the invariances and the diagonal}{}{}}
\newlabel{sec:S-contact-image}{{S7.3}{27}{The momentum image, step by step}{}{}}
\newlabel{eq:S-contact-composition}{{S7.9}{27}{Step 1: the composition is the second area derivative}{}{}}
\newlabel{eq:S-contact-gradient-coord}{{S7.10}{28}{Step 3: one gradient insertion}{}{}}
\newlabel{eq:S-contact-product}{{S7.11}{28}{Step 5: the product of the two insertions}{}{}}
\newlabel{eq:S-contact-op}{{S7.12}{29}{Step 7: the rule at the mark}{}{}}
\newlabel{eq:S-contact-ordered}{{S7.13}{29}{Step 7: the rule at the mark}{}{}}
\newlabel{sec:S-contact-rotation}{{S7.4}{30}{Benchmark: the uniform rotation}{}{}}
\newlabel{eq:S-contact-rot-cov}{{S7.14}{30}{Representation and convention}{}{}}
\newlabel{eq:S-contact-rot-sawtooth}{{S7.15}{30}{Representation and convention}{}{}}
\newlabel{eq:S-contact-refined-F}{{S7.16}{30}{Refinement conventions}{}{}}
\newlabel{eq:S-contact-rot-pairs}{{S7.17}{31}{Without refinement}{}{}}
\newlabel{eq:S-contact-rot-totals}{{S7.18}{31}{Without refinement}{}{}}
\newlabel{lem:S-contact-local}{{S7.1}{32}{Local bounds on the terms at the mark}{}{}}
\newlabel{eq:S-contact-local}{{S7.19}{32}{Local bounds on the terms at the mark}{}{}}
\newlabel{eq:S-contact-adj}{{S7.20}{33}{The Euler states}{}{}}
\newlabel{rem:S-contact-locations}{{S7.2}{33}{Typical locations}{}{}}
\newlabel{sec:two-dimensional}{{S8}{34}{Two dimensions: the complex rotating polygon}{}{}}
\newlabel{eq:2d-rescaling}{{S8.1}{34}{Two dimensions: the complex rotating polygon}{}{}}
\newlabel{eq:2d-full-rescaled}{{S8.2}{34}{Two dimensions: the complex rotating polygon}{}{}}
\newlabel{eq:2d-arithmetic-parameters}{{S8.3}{34}{Rational angles and the logarithmic rotation}{}{}}
\newlabel{prop:2d-complex-rotation}{{S8.1}{35}{Complex planar Euler trajectory}{}{}}
\newlabel{eq:2d-complex-rotation}{{S8.4}{35}{Complex planar Euler trajectory}{}{}}
\newlabel{eq:2d-invariants}{{S8.5}{35}{Complex planar Euler trajectory}{}{}}
\newlabel{eq:2d-complex-phase-average}{{S8.6}{35}{A real representative of the orientation average}{}{}}
\newlabel{prop:2d-phase-shift}{{S8.2}{35}{Moving the orientation contour}{}{}}
\newlabel{eq:2d-real-phase-average}{{S8.7}{35}{Moving the orientation contour}{}{}}
\newlabel{sec:two-dimensional-rigidity}{{S9}{36}{Two dimensions: rigidity on the circle}{}{}}
\newlabel{eq:2d-angle-gaps}{{S9.1}{36}{Two dimensions: rigidity on the circle}{}{}}
\newlabel{prop:2d-fixed-circle-rigidity}{{S9.1}{36}{Local rigidity of real gaps}{}{}}
\newlabel{sec:2d-positivity}{{S10}{36}{Two dimensions: the vorticity correlation violates positivity}{}{}}
\newlabel{eq:2d-polygon-spectrum}{{S10.1}{36}{Two dimensions: the vorticity correlation violates positivity}{}{}}
\newlabel{eq:2d-two-insertion-sign}{{S10.2}{37}{Two dimensions: the vorticity correlation violates positivity}{}{}}
\newlabel{eq:2d-corrected-pair}{{S10.3}{37}{Two dimensions: the vorticity correlation violates positivity}{}{}}
\newlabel{eq:2d-zero-separation}{{S10.4}{37}{Two dimensions: the vorticity correlation violates positivity}{}{}}
\newlabel{prop:2d-rejected}{{S10.1}{37}{The planar solution fails the finite-cutoff enstrophy test}{}{}}
\newlabel{sec:2d-cond}{{S10.1}{38}{The conditional correlation}{}{}}
\newlabel{eq:2d-cond-Q}{{S10.5}{38}{The conditional correlation}{}{}}
\newlabel{eq:2d-cond-mid}{{S10.6}{38}{The conditional correlation}{}{}}
\newlabel{eq:2d-cond-split}{{S10.7}{38}{The conditional correlation}{}{}}
\newlabel{eq:2d-cond-zero}{{S10.8}{39}{The conditional correlation}{}{}}
\newlabel{eq:2d-cond-neumann}{{S10.9}{39}{The conditional correlation}{}{}}
\newlabel{eq:2d-cond-limit}{{S10.10}{39}{The conditional correlation}{}{}}
\newlabel{eq:2d-cond-asym}{{S10.11}{39}{The conditional correlation}{}{}}
\newlabel{prop:2d-conditional}{{S10.2}{40}{The conditional correlation of the planar solution is negative}{}{}}
\newlabel{eq:2d-cond-transforms}{{S10.12}{40}{The conditional correlation}{}{}}
\newlabel{eq:2d-cond-measure}{{S10.13}{41}{The conditional correlation}{}{}}
\newlabel{sec:S-2d}{{S11}{41}{Two dimensions: the complex rotation, its average and the conditional correlation}{}{}}
\newlabel{eq:2d-stretch}{{S11.1}{41}{Two dimensions: the complex rotation, its average and the conditional correlation}{}{}}
\newlabel{rem:2d-growth}{{S11.2}{42}{Where the growth goes}{}{}}
\newlabel{eq:2d-growth-z}{{S11.2}{42}{Where the growth goes}{}{}}
\newlabel{eq:2d-growth-J0}{{S11.3}{42}{Where the growth goes}{}{}}
\newlabel{sec:S-2d-cond}{{S11.1}{43}{The conditional correlation: derivations and numbers}{}{}}
\newlabel{eq:S-2d-marks}{{S11.4}{43}{The phases at the marks for any polygon}{}{}}
\newlabel{eq:S-2d-mellin}{{S11.5}{45}{The Mellin transforms and the asymptotes}{}{}}
\newlabel{eq:S-2d-F}{{S11.6}{46}{Positive values at finite $N$}{}{}}
\newlabel{sec:S-2d-rigidity}{{S12}{47}{Two dimensions: proof of rigidity on the circle}{}{}}
\newlabel{eq:2d-gap-equation}{{S12.1}{47}{Two dimensions: proof of rigidity on the circle}{}{}}
\newlabel{eq:2d-phase-equation}{{S12.2}{47}{Two dimensions: proof of rigidity on the circle}{}{}}
\newlabel{eq:2d-gap-derivatives}{{S12.3}{48}{Two dimensions: proof of rigidity on the circle}{}{}}
\newlabel{eq:2d-linear-difference}{{S12.4}{48}{The formal square mode}{}{}}
\newlabel{eq:2d-linear-sum}{{S12.5}{48}{The formal square mode}{}{}}
\newlabel{eq:2d-formal-square-mode}{{S12.6}{48}{The formal square mode}{}{}}
\newlabel{eq:2d-square-obstruction}{{S12.7}{48}{The formal square mode}{}{}}
\newlabel{eq:2d-varying-square}{{S12.8}{48}{A fixed radius is stronger than a varying one}{}{}}
\newlabel{sec:S-3d-odd}{{S13}{49}{Three dimensions: the odd states and the counting measure}{}{}}
\newlabel{eq:3d-all-winding-collapse}{{S13.1}{49}{Three dimensions: the odd states and the counting measure}{}{}}
\newlabel{eq:3d-exact-all-winding-Z}{{S13.2}{49}{Three dimensions: the odd states and the counting measure}{}{}}
\newlabel{sec:3d-grand}{{S14}{49}{Three dimensions: the grand canonical ensemble and the dominance of zero winding}{}{}}
\newlabel{eq:grand-ratio}{{S14.1}{50}{Three sectors}{}{}}
\newlabel{sec:S-3d}{{S15}{51}{Three dimensions: the real phase representative and the counting}{}{}}
\newlabel{sec:S-3d-real}{{S15.1}{52}{The real phase representative and its scope}{}{}}
\newlabel{eq:3d-real-phase}{{S15.2}{52}{The real phase representative and its scope}{}{}}
\newlabel{sec:S-3d-main}{{S15.2}{52}{The statistical weight: invariance and the limit}{}{}}
\newlabel{sec:rigidity3d}{{S16}{53}{Three dimensions: rigidity of the odd and even Euler ensembles}{}{}}
\newlabel{eq:rig3d-fixed-lift}{{S16.1}{53}{Rigidity of the complex Euler polygon}{}{}}
\newlabel{prop:rig3d}{{S16.1}{53}{Rigidity of the fixed complex lift}{}{}}
\newlabel{prop:rig3d-even}{{S16.2}{53}{Rigidity of the fixed complex lift for even $N$}{}{}}
\newlabel{rem:rig3d-family}{{S16.3}{54}{The family of zero-winding fixed points}{}{}}
\newlabel{rem:rig3d-linear}{{S16.4}{54}{The unrestricted linearization}{}{}}
\newlabel{eq:rig3d-invariant-measure}{{S16.2}{55}{Invariance of the selected ensemble}{}{}}
\newlabel{sec:S-3d-rigidity}{{S17}{55}{Three dimensions: proofs of rigidity}{}{}}
\newlabel{eq:rig3d-operators}{{S17.1}{55}{Three dimensions: proofs of rigidity}{}{}}
\newlabel{eq:rig3d-rescaling}{{S17.2}{55}{Three dimensions: proofs of rigidity}{}{}}
\newlabel{eq:rig3d-inverse}{{S17.3}{55}{Three dimensions: proofs of rigidity}{}{}}
\newlabel{eq:rig3d-complex-defects}{{S17.4}{55}{Three dimensions: proofs of rigidity}{}{}}
\newlabel{eq:rig3d-null-reduction}{{S17.5}{56}{Three dimensions: proofs of rigidity}{}{}}
\newlabel{eq:rig3d-normal-equation}{{S17.6}{56}{Three dimensions: proofs of rigidity}{}{}}
\newlabel{sec:S-rig3d-even}{{S17.1}{56}{Even \texorpdfstring {$N$}{N}}{}{}}
\newlabel{eq:rig3d-real-rescaled}{{S17.7}{56}{Exact angular compatibility of the real diffusive representative}{}{}}
\newlabel{eq:rig3d-circle-angles}{{S17.8}{56}{Exact angular compatibility of the real diffusive representative}{}{}}
\newlabel{eq:rig3d-angular-midpoint}{{S17.9}{56}{Exact angular compatibility of the real diffusive representative}{}{}}
\newlabel{eq:rig3d-angular-compatibility}{{S17.10}{57}{Exact angular compatibility of the real diffusive representative}{}{}}
\newlabel{eq:rig3d-linear-compatibility}{{S17.11}{57}{Exact angular compatibility of the real diffusive representative}{}{}}
\newlabel{eq:rig3d-angular-pencil}{{S17.12}{57}{Exact angular compatibility of the real diffusive representative}{}{}}
\newlabel{eq:rig3d-even-period-two}{{S17.13}{57}{Even $N$, real representative}{}{}}
\newlabel{sec:rig3d-neutral}{{S17.3}{57}{Radial directions, spherical confinement, and neutral shapes}{}{}}
\newlabel{eq:rig3d-telescopic-bound}{{S17.14}{57}{Radial directions, spherical confinement, and neutral shapes}{}{}}
\newlabel{eq:rig3d-time-origin}{{S17.15}{58}{Radial directions, spherical confinement, and neutral shapes}{}{}}
\newlabel{eq:rig3d-coupled-defects}{{S17.16}{58}{Radial directions, spherical confinement, and neutral shapes}{}{}}
\newlabel{sec:S-hairpin}{{S18}{58}{Three dimensions: the vorticity correlation, details}{}{}}
\newlabel{rem:3d-normal-only}{{S18.1}{58}{The normal component and the earlier calculations}{}{}}
\newlabel{eq:3d-unrestricted-cot-square}{{S18.1}{59}{Zero separation in the odd ensemble}{}{}}
\newlabel{eq:3d-binomial-moment-identities}{{S18.2}{59}{Zero separation in the odd ensemble}{}{}}
\newlabel{eq:3d-YN}{{S18.3}{59}{Zero separation in the odd ensemble}{}{}}
\newlabel{rem:S-small-angles}{{S18.2}{60}{Why the small angles of Ref.~\cite {migdal2024quantum} do not contribute}{}{}}
\newlabel{sec:S-cond-remarks}{{S19}{61}{The conditional correlation: the hairpin amplitude, the literal ratio and other orders}{}{}}
\newlabel{sec:hairpin-not-one}{{S19.1}{61}{The hairpin factor is not one}{}{}}
\newlabel{eq:hp-stokes}{{S19.1}{61}{Coordinate space}{}{}}
\newlabel{eq:hp-phase}{{S19.2}{62}{Momentum space}{}{}}
\newlabel{sec:S-cond-translation}{{S19.2}{62}{The planar vorticity is a translation}{}{}}
\newlabel{sec:S-cond-bulk}{{S19.3}{62}{The literal ratio and the bulk of the hairpin}{}{}}
\newlabel{eq:cond-bulk-mid}{{S19.3}{62}{The literal ratio and the bulk of the hairpin}{}{}}
\newlabel{sec:S-cond-factorization}{{S19.4}{63}{A heuristic factorization}{}{}}
\newlabel{eq:cond-factorization}{{S19.4}{63}{A heuristic factorization}{}{}}
\newlabel{sec:S-cond-orders}{{S19.5}{63}{The other orders of the averages}{}{}}
\newlabel{eq:cond-def-r}{{S19.5}{63}{The other orders of the averages}{}{}}
\newlabel{sec:S-cond-odd-zero}{{S19.6}{64}{The odd ensemble at zero separation}{}{}}
\newlabel{sec:S-hairpin-main}{{S20}{65}{The vorticity correlation: closure sums, the hairpin factor and the finite-\texorpdfstring {$N$}{N} ratio}{}{}}
\newlabel{sec:S-hp-closure}{{S20.1}{65}{The contraction, the conventions, the pair weight and the Hankel inversion}{}{}}
\newlabel{eq:3d-vorticity-contraction}{{S20.1}{65}{The contraction, the conventions, the pair weight and the Hankel inversion}{}{}}
\newlabel{eq:3d-closure-sums}{{S20.2}{65}{The contraction, the conventions, the pair weight and the Hankel inversion}{}{}}
\newlabel{eq:3d-pair-weight}{{S20.3}{65}{The contraction, the conventions, the pair weight and the Hankel inversion}{}{}}
\newlabel{eq:3d-vorticity-correlation}{{S20.4}{66}{The contraction, the conventions, the pair weight and the Hankel inversion}{}{}}
\newlabel{eq:3d-hankel-inversion}{{S20.5}{66}{The contraction, the conventions, the pair weight and the Hankel inversion}{}{}}
\newlabel{sec:S-hp-factor}{{S20.2}{66}{The hairpin factor: the bound, the variance and the values}{}{}}
\newlabel{sec:S-hp-finiteN}{{S20.3}{67}{The conditional correlation at finite \texorpdfstring {$N$}{N}}{}{}}
\newlabel{eq:3d-formal-dissipation}{{S20.6}{67}{The pendulum limit}{}{}}
\newlabel{sec:3d-transfer}{{S21}{68}{Three dimensions: an exact transfer-matrix formula}{}{}}
\newlabel{eq:3d-transfer-marks}{{S21.1}{68}{Three dimensions: an exact transfer-matrix formula}{}{}}
\newlabel{eq:3d-transfer-formula}{{S21.2}{68}{Three dimensions: an exact transfer-matrix formula}{}{}}
\newlabel{sec:S-fermion-main}{{S22}{68}{The fermionic trace: derivations, quantum thimbles and the chain of representations}{}{}}
\newlabel{eq:fermion-markov}{{S22.1}{69}{The Markov product and the counting}{}{}}
\newlabel{eq:fermion-markov-product}{{S22.2}{69}{The Markov product and the counting}{}{}}
\newlabel{eq:fermion-sector-average}{{S22.3}{69}{The Markov product and the counting}{}{}}
\newlabel{sec:S-fermion-transfer}{{S22.3}{69}{The transfer operator at a rational angle}{}{}}
\newlabel{eq:fermion-insertion}{{S22.4}{69}{The transfer operator at a rational angle}{}{}}
\newlabel{eq:fermion-two-spin}{{S22.5}{70}{The transfer operator at a rational angle}{}{}}
\newlabel{eq:fermion-arc-spectral}{{S22.6}{70}{The evolution along an arc and the quantum thimbles}{}{}}
\newlabel{sec:S-fermion-chain}{{S22.6}{71}{From the fermionic trace to one-dimensional quantum mechanics}{}{}}
\newlabel{sec:S-fermion}{{S23}{71}{The fermionic trace: the odd ensemble, the spectral equation and tests}{}{}}
\newlabel{eq:3d-half-turn}{{S23.1}{72}{The odd ensemble}{}{}}
\newlabel{eq:fermion-normal-currents}{{S23.2}{72}{The odd ensemble}{}{}}
\newlabel{sec:S-odd-cond}{{S23.2}{72}{The odd ensemble: the conditional correlation in the limit}{}{}}
\newlabel{eq:S-odd-orders}{{S23.3}{73}{The two orders}{}{}}
\newlabel{eq:S-odd-measure}{{S23.4}{74}{The half-turn measure}{}{}}
\newlabel{eq:S-odd-ZG}{{S23.5}{74}{The half-turn measure}{}{}}
\newlabel{eq:S-odd-small}{{S23.6}{75}{Small separation}{}{}}
\newlabel{eq:S-odd-small-h}{{S23.7}{75}{Small separation}{}{}}
\newlabel{eq:S-odd-gauss}{{S23.8}{76}{The spectrum at a fixed projected separation}{}{}}
\newlabel{eq:S-odd-plateau}{{S23.9}{76}{The spectrum at a fixed separation}{}{}}
\newlabel{eq:fermion-monodromy}{{S23.10}{77}{The spectrum of the transfer operator}{}{}}
\newlabel{eq:fermion-spectral}{{S23.11}{77}{The spectrum of the transfer operator}{}{}}
\newlabel{rem:fermion-bethe}{{S23.1}{78}{Is there a Bethe ansatz?}{}{}}
\newlabel{eq:3d-planar-identity}{{S23.12}{78}{The planar insertion}{}{}}
\newlabel{eq:fermion-planar-jump}{{S23.13}{78}{The planar insertion}{}{}}
\newlabel{eq:3d-one-label}{{S23.14}{78}{The planar insertion}{}{}}
\newlabel{eq:3d-parity-average}{{S23.15}{78}{The planar insertion}{}{}}
\newlabel{eq:3d-vertex-operators}{{S23.16}{78}{The planar insertion}{}{}}
\newlabel{sec:S-even-steps}{{S24}{79}{The source function of the even ensemble, step by step}{}{}}
\newlabel{eq:ev-pendulum}{{S24.1}{81}{Step 3: the hairpin factor becomes two pendulums}{}{}}
\newlabel{eq:S-ev-bands}{{S24.2}{83}{Step 9: the result}{}{}}
\newlabel{sec:S-even-arith-steps}{{S24.11}{84}{The labels near $\beta =\pi $}{}{}}
\newlabel{eq:ev-density}{{S24.3}{84}{The labels near $\beta =\pi $}{}{}}
\newlabel{sec:S-floquet-steps}{{S24.12}{84}{The Floquet form, step by step}{}{}}
\newlabel{eq:ev-split}{{S24.4}{84}{First: the square of a sum of two energies is an integral over an imaginary energy}{}{}}
\newlabel{eq:ev-floquet-kernel}{{S24.5}{85}{Second: the integral over the Bloch angle is a trace on the whole line}{}{}}
\newlabel{eq:S-Z-floquet}{{S24.6}{85}{The partition function}{}{}}
\newlabel{sec:S-asym-steps}{{S24.13}{86}{The asymptotes of the source}{}{}}
\newlabel{eq:S-end-a}{{S24.7}{86}{The end layers as quadratures}{}{}}
\newlabel{eq:S-end-p}{{S24.8}{86}{The end layers as quadratures}{}{}}
\newlabel{sec:pendulum}{{S25}{88}{The quantum pendulum: bands, Bloch states and the source}{}{}}
\newlabel{eq:pend-H}{{S25.1}{88}{Bands and Bloch states}{}{}}
\newlabel{eq:3d-fourier-matrix}{{S25.2}{88}{Bands and Bloch states}{}{}}
\newlabel{eq:pend-deep}{{S25.3}{88}{Bands and Bloch states}{}{}}
\newlabel{fig:pendulum}{{S1}{89}{The pendulum \eqref {eq:pend-H}. (a) The bands $\lambda _m(\alpha )$, $0\le \alpha \le 1$ (shaded, $m=0,\dots ,9$), against $\omega _L=h/4L$, with the barrier $\omega _L^2/2$ (dashed) and the deep-well levels \eqref {eq:pend-deep} (dotted). (b) The Bloch densities $|\psi _{m,\alpha }(\theta )|^2$ of the four lowest bands at $\omega _L=4$, at $\alpha =0$ (solid) and $\alpha =1$ (dashed), shifted vertically; the potential is shown below. The two lowest states lie below the barrier and are localized in the wells; the third is at the barrier, and the fourth is extended}{}{}}
\newlabel{eq:pend-bessel}{{S25.4}{89}{Matrix elements of the tip operators}{}{}}
\newlabel{eq:pend-duhamel}{{S25.5}{90}{The mean-field part}{}{}}
\newlabel{eq:pend-Sf}{{S25.6}{90}{The mean-field part}{}{}}
\newlabel{sec:pend-deep}{{S25.4}{90}{Deep wells}{}{}}
\newlabel{rem:3d-tba}{{S25.1}{91}{Exact WKB, the Mathieu TBA and Baxter's equation}{}{}}
\newlabel{sec:pend-floquet}{{S25.5}{91}{The Floquet form of the source}{}{}}
\newlabel{eq:pf-SB}{{S25.7}{91}{The Floquet form of the source}{}{}}
\newlabel{eq:pf-D}{{S25.8}{92}{The Floquet form of the source}{}{}}
\newlabel{eq:pf-T}{{S25.9}{92}{The Floquet form of the source}{}{}}
\newlabel{eq:pf-cell}{{S25.10}{92}{The Bloch angle}{}{}}
\newlabel{eq:pf-floquet}{{S25.11}{92}{The Bloch angle}{}{}}
\newlabel{eq:pf-Z-sum}{{S25.12}{93}{The cell trace of the partition function}{}{}}
\newlabel{eq:pf-riccati-kernel}{{S25.13}{93}{The cell trace of the partition function}{}{}}
\newlabel{eq:pf-Z-riccati}{{S25.14}{93}{The cell trace of the partition function}{}{}}
\newlabel{eq:pf-J-riccati}{{S25.15}{93}{The cell trace of the partition function}{}{}}
\newlabel{sec:S-cond}{{S26}{95}{The conditional state of the hairpin: formulas and checks}{}{}}
\newlabel{sec:S-cond-main}{{S26.1}{95}{The Gibbs state: the kind of theory, the gauge of the thermostat and the numerator}{}{}}
\newlabel{sec:S-cond-checks}{{S26.2}{96}{The partition function of the hairpin}{}{}}
\newlabel{eq:S-cond-path}{{S26.1}{97}{The path measure}{}{}}
\newlabel{eq:S-cond-free}{{S26.2}{98}{Small $h$}{}{}}
\newlabel{eq:cond-resolvent}{{S26.3}{98}{The endpoint operators}{}{}}
\newlabel{eq:cond-kernel}{{S26.4}{99}{The cell formula}{}{}}
\newlabel{eq:cond-cell}{{S26.5}{99}{The cell formula}{}{}}
\newlabel{eq:S-cond-large}{{S26.6}{99}{Values and asymptotes}{}{}}
\newlabel{sec:S-cond-literal}{{S26.3}{100}{The literal conditioning}{}{}}
\newlabel{eq:S-cond-bulk}{{S26.7}{101}{The bulk at finite $N$}{}{}}
\newlabel{sec:S-even-formulas}{{S27}{102}{The even ensemble at zero winding: explicit formulas}{}{}}
\newlabel{eq:ev-PQ}{{S27.1}{102}{The operators}{}{}}
\newlabel{eq:ev-spin-ops}{{S27.2}{102}{The operators}{}{}}
\newlabel{eq:ev-S2}{{S27.3}{103}{The operators}{}{}}
\newlabel{eq:ev-small-ratio}{{S27.4}{103}{Small $h$}{}{}}
\newlabel{sec:S-even}{{S28}{103}{The even ensemble at zero winding: exact sums and tests}{}{}}
\newlabel{sec:S-labels}{{S28.1}{103}{The sum over the rational angles}{}{}}
\newlabel{sec:S-valid}{{S28.2}{104}{Test of the continuum formula}{}{}}
\newlabel{sec:S-arith}{{S29}{104}{The arithmetic at zero winding}{}{}}
\newlabel{eq:ev-perron}{{S29.1}{105}{The arithmetic at zero winding}{}{}}
\newlabel{rem:ev-zeros}{{S29.1}{105}{Where the Riemann zeros go}{}{}}
\newlabel{eq:ev-theta}{{S29.2}{105}{Where the Riemann zeros go}{}{}}
\newlabel{fig:ev-arith}{{S2}{106}{The arithmetic of the zero-winding labels. (a) The density of labels near $\beta =\pi $, in units of its mean, against $X=N|\beta -\pi |/\pi $: the totient staircase \eqref {eq:ev-density} (line) and the exact labels at $N=20000$ in bins of width $0.1$ (circles); in the limit only the flat mean survives. (b) The finite-$N$ form factor of Remark~\ref {rem:ev-zeros} after subtraction of its real poles, $[R(t)-1-\pi ^2t/18-\dots ]/t^{3/4}$ (circles), and the contribution of the nontrivial zeros of $\zeta $ (line), dominated by the first zero}{}{}}
\newlabel{eq:ev-Rmellin}{{S29.3}{106}{Where the Riemann zeros go}{}{}}
\newlabel{sec:ev-eval}{{S30}{106}{Evaluation of the source function}{}{}}
\newlabel{sec:S-even-details}{{S31}{108}{The even ensemble at zero winding: details}{}{}}
\newlabel{fig:ev-G0}{{S3}{111}{The conditional source $C(h)=g/\Pi $ (solid), in units of $1/N$, with its numerator $g=h\widehat G$ (dashed) and the partition function $\Pi =h\widehat Z$ (dash-dotted), against $h$ on a logarithmic axis, $10^{-3}\le h\le 10^3$, with a linear vertical axis: lines through the Floquet quadratures \eqref {eq:ev-floquet} and \eqref {eq:cond-floquet}. Dotted: the limits $\frac 18$, $\sqrt \pi /32$ and $\sqrt \pi /4$ as $h\to 0$. Thin solid lines: the laws $C\simeq \frac 18-(4a_{1/2}/\sqrt \pi )h^{1/2}$ at small $h$, Eq.~\eqref {eq:ev-small}, and $\Pi \simeq (\log h+\bar \kappa )/(4\sqrt {2\pi })+c_0/h$ at large $h$, Eq.~\eqref {eq:ev-large}. Inset: $10^4\,C(h)$ on $1.2<h<2.5$, with linear axes and the line $C=0$; $C$ is negative on $\QCDIPLO <h<\QCDIPHI $, with the minimum $\QCMIN $ at $h\simeq \QCMINH $; the open circles mark the zeros and the dot the minimum}{}{}}
\newlabel{eq:ev-small-a}{{S31.1}{112}{Small $h$}{}{}}
\newlabel{sec:S-tail-closed}{{S31.4}{113}{Closed forms of the large-\texorpdfstring {$h$}{h} constants}{}{}}
\newlabel{eq:S-tail-closed}{{S31.2}{113}{Closed forms of the large-\texorpdfstring {$h$}{h} constants}{}{}}
\newlabel{eq:S-tail-closed-a2}{{S31.3}{113}{Closed forms of the large-\texorpdfstring {$h$}{h} constants}{}{}}
\newlabel{tab:S-tail-closed}{{S1}{114}{The closed forms \eqref {eq:S-tail-closed} and \eqref {eq:S-tail-closed-a2} of Ref.~\cite {JiangMigdalLean2026} against the values fitted to the Floquet values in this paper}{}{}}
\newlabel{sec:S-whole-evidence}{{S31.5}{114}{The evidence over the whole ensemble}{}{}}
\newlabel{sec:ev-whole}{{S32}{115}{The whole ensemble}{}{}}
\newlabel{sec:S-mc}{{S33}{116}{Direct simulation of the ensemble by a Markov chain}{}{}}
\newlabel{eq:mc-markov}{{S33.1}{117}{The algorithm}{}{}}
\newlabel{eq:mc-estimator}{{S33.2}{117}{The algorithm}{}{}}
\newlabel{sec:S-finiteN}{{S34}{119}{The finite-$N$ test of the conditional ratio}{}{}}
\newlabel{eq:S-finiteN-limits}{{S34.1}{119}{The finite-$N$ test of the conditional ratio}{}{}}
\newlabel{sec:S-finiteN-proof}{{S34.1}{123}{A proof of the limits}{}{}}
\newlabel{eq:S-fp-theorem}{{S34.2}{123}{A proof of the limits}{}{}}
\newlabel{eq:S-fp-pairs}{{S34.3}{123}{Pairs of spins}{}{}}
\newlabel{eq:S-fp-martingale}{{S34.4}{123}{Pairs of spins}{}{}}
\newlabel{eq:S-fp-trace}{{S34.5}{124}{From the walk to the pendulums}{}{}}
\newlabel{eq:S-fp-lower}{{S34.6}{124}{The pendulum integral}{}{}}
\newlabel{sec:S-spectrum-details}{{S35}{125}{The energy spectrum: details}{}{}}
\newlabel{sec:S-renorm}{{S35.1}{125}{Renormalization and the turbulent viscosity}{}{}}
\newlabel{eq:3d-renorm}{{S35.1}{126}{The renormalization}{}{}}
\newlabel{sec:S-weak-limit}{{S35.2}{129}{The weak limit and the chain of quadratures}{}{}}
\newlabel{eq:ev-weak-limit}{{S35.2}{129}{The weak limit and the chain of quadratures}{}{}}
\newlabel{eq:ev-chain}{{S35.3}{130}{The weak limit and the chain of quadratures}{}{}}
\newlabel{eq:ev-IR-next}{{S35.4}{131}{Infrared}{}{}}
\newlabel{sec:ev-mellin}{{S35.4}{133}{The Mellin amplitude}{}{}}
\newlabel{eq:ev-mellin}{{S35.5}{133}{The Mellin amplitude}{}{}}
\newlabel{eq:3d-energy-above-k0}{{S35.6}{134}{Time dependence: the energy above a fixed wave number}{}{}}
\newlabel{eq:3d-decay-index}{{S35.7}{135}{Time dependence: the energy above a fixed wave number}{}{}}
\newlabel{sec:S-energy-balance}{{S35.6}{135}{The energy balance}{}{}}
\newlabel{eq:S-balance}{{S35.8}{135}{The energy balance}{}{}}
\newlabel{eq:S-KH}{{S35.9}{136}{The Kolmogorov tensor}{}{}}
\newlabel{sec:S-open}{{S36}{137}{What remains to be settled}{}{}}
\newlabel{rem:3d-dissipation}{{S36.1}{137}{The dissipation lies outside the limit at fixed $K$}{}{}}
\newlabel{eq:3d-bulk-dissipation}{{S36.1}{137}{The dissipation lies outside the limit at fixed $K$}{}{}}
\newlabel{rem:3d-energy-normalization}{{S36.2}{138}{Energy normalization is postponed}{}{}}
\newlabel{rem:3d-matching}{{S36.3}{138}{Convergence and matching}{}{}}
\newlabel{rem:ev-open}{{S36.4}{138}{What the conditional spectrum rests on}{}{}}
\newlabel{sec:S-spectrum}{{S37}{139}{The spectrum: selected values and accuracy}{}{}}
\newlabel{sec:S-annealed}{{S37.1}{140}{The annealed order: the spectrum, the correlation and the finite-size effects}{}{}}
\newlabel{eq:S-ann-c}{{S37.1}{140}{The correlation}{}{}}
\newlabel{eq:S-ann-small}{{S37.2}{140}{The correlation}{}{}}
\newlabel{eq:S-ann-large}{{S37.3}{141}{The correlation}{}{}}
\newlabel{eq:S-ann-P}{{S37.4}{141}{The transform}{}{}}
\newlabel{eq:S-ann-IR}{{S37.5}{142}{The laws}{}{}}
\newlabel{eq:S-ann-I}{{S37.6}{143}{Finite size}{}{}}
\newlabel{sec:S-osc-derivation}{{S38}{144}{Oscillations in coordinate space: derivations}{}{}}
\newlabel{eq:osc-source-cond}{{S38.1}{145}{The amplitude}{}{}}
\newlabel{eq:osc-a2}{{S38.2}{145}{The amplitude}{}{}}
\newlabel{eq:osc-lighthill}{{S38.3}{145}{The amplitude}{}{}}
\newlabel{eq:osc-mellin}{{S38.4}{146}{Small separation}{}{}}
\newlabel{fig:osc-index}{{S4}{148}{Effective indices of the correlation functions of the conditional state, against $\log (r/L)$. (a) The index $n_\omega =-\partial \log C_\omega /\partial \log r$ of the vorticity correlation (line); the same with the oscillating term of the source removed (dashed), and the envelope $n_\omega ^{\rm reg}\pm 2\sqrt \pi \,|D|/[\Pi (R/\sqrt 2)\,R^2c_{\rm reg}(R)]$ of the oscillation, Eq.~\eqref {eq:osc-n} (dotted), both for $r\ge 4\sqrt 2\,L$: the oscillating term is removed for $h>2$, fully from $h=4$, and the Abel average reaches $h=R/\sqrt 2$. The horizontal line marks $2$. The oscillation decays asymptotically as $1/\log ^2(r/L)$. (b) The index $\zeta _2$ of the velocity structure function \eqref {eq:osc-zeta} (line); its small-$R$ law $2-\QCOZSMALL \,R^{1/2}$ (dashed); its large-$R$ law, the first relation of \eqref {eq:osc-S-large} divided by its integral, with the constant of integration taken from the computed $\mathcal S$ at $R=10^4$ (dotted); the asymptote $2/\log R$, which is reached only logarithmically (thin dotted); and the index $\zeta _{LL}$ of the longitudinal function (dash-dotted). The horizontal line marks $2/3$}{}{}}
\newlabel{eq:osc-DC}{{S38.5}{149}{The velocity structure function}{}{}}
\newlabel{eq:osc-zeta-osc}{{S38.6}{149}{The velocity structure function}{}{}}
\newlabel{sec:S-osc}{{S39}{150}{Oscillations in coordinate space: computations}{}{}}
\newlabel{fig:osc-origin}{{S5}{151}{The origin of the wave. (a) The oscillating part of the source, $h^{5/2}[h\widehat G-s(h)]$ with $s$ the fitted non-oscillating part of \eqref {eq:ev-large}, with its next orders in $1/h$, for the computed values $6\le h\le 80$, divided by its amplitude $|D_{\rm eff}|$ and plotted against its phase $\phi $ modulo $2\pi $: open circles with the stationary-phase amplitude of \eqref {eq:osc-source}, $D_{\rm eff}=D$ and $\phi =2h+\arg D$; filled circles, coloured by $\log h$, with the next order, $D_{\rm eff}=D+D_1/h$; the line is $\cos \phi $. (b) The oscillating part of the conditional vorticity correlation \eqref {eq:ev-corr}, in units of $10^{-3}$: the difference between the correlations computed with the full source and with its oscillating part removed, multiplied by $R^3\,h\widehat Z(h)$ at $h=R/\sqrt 2$, minus its average over one period (line), the asymptotic form \eqref {eq:osc-c} (dashed), and the same with $D+\sqrt 2D_1/R$ in place of $D$ (dotted); the removal is complete for $r>4\sqrt 2\,L$, and for $R\ge 6$ the subtraction of the non-oscillating part computed from the moments of the removed term, as in the table of this section, gives the same curve to about $2\%$ of $|D|$. The period is $\pi $ in $h$ and $2\pi /\sqrt 2$ in $R=r/L$: the Abel integral reads the source, and the partition function, at $h=R/\sqrt 2$}{}{}}
\newlabel{sec:S-limits-full}{{S40}{152}{The scaling limits: layers, exponents and the choice}{}{}}
\newlabel{sec:S-limits}{{S41}{154}{The scaling limits of the even ensemble}{}{}}
\newlabel{eq:S-lim-s2}{{S41.1}{155}{The Gaussian layer}{}{}}
\newlabel{eq:S-lim-clt}{{S41.2}{155}{The Gaussian layer}{}{}}
\newlabel{eq:lim-P1}{{S41.3}{155}{The function $P_1$}{}{}}
\newlabel{eq:lim-F}{{S41.4}{155}{The function $P_1$}{}{}}
\newlabel{eq:lim-P1-asym}{{S41.5}{155}{The function $P_1$}{}{}}
\newlabel{eq:S-lim-VN}{{S41.6}{156}{The function $P_1$}{}{}}
\newlabel{eq:S-lim-Fuv}{{S41.7}{156}{The function $P_1$}{}{}}
\newlabel{sec:S-small-angles}{{S42}{158}{The small-angle layer is exponentially small}{}{}}
\newlabel{eq:S-sa-E}{{S42.1}{158}{The result}{}{}}
\newlabel{sec:S-sa-mirror}{{S42.1}{158}{The mirror symmetry \texorpdfstring {$\beta \to 2\pi -\beta $}{beta -> 2 pi - beta}}{}{}}
\newlabel{eq:S-sa-mirror}{{S42.2}{158}{The mirror symmetry \texorpdfstring {$\beta \to 2\pi -\beta $}{beta -> 2 pi - beta}}{}{}}
\newlabel{eq:S-sa-label}{{S42.3}{159}{One label}{}{}}
\newlabel{eq:S-sa-arc}{{S42.4}{159}{The arc operators}{}{}}
\newlabel{eq:S-sa-decay}{{S42.5}{159}{The arc operators}{}{}}
\newlabel{prop:S-sa-reduction}{{S42.1}{159}{Reduction to single arcs}{}{}}
\newlabel{eq:S-sa-bound}{{S42.6}{159}{Reduction to single arcs}{}{}}
\newlabel{eq:S-sa-layer}{{S42.7}{160}{Consequences}{}{}}
\newlabel{sec:S-sa-arcs}{{S42.3}{161}{The decay along one arc}{}{}}
\newlabel{prop:S-sa-arcs}{{S42.2}{161}{One arc}{}{}}
\newlabel{sec:S-sa-numerics}{{S42.5}{163}{Numerical checks}{}{}}
\newlabel{fig:S-small-angles}{{S6}{165}{The small-angle layer. (a) The arc operator on the lattice: $-\log \rho (T_\lambda )/\gamma _0$ against $\beta \sqrt \lambda $ at fixed $\lambda \beta $. (b) $\sum |W_{N,p/q}|$ over the layer $\beta \le 3/\sqrt N$ (points) and the whole source $W_N(h)$ (lines). (c) Every small-angle label computed: $\log _{10}|W_{N,p/q}|$ against $E_{p/q}/2$, Eq.~\eqref {eq:S-sa-E}; dashed: $e^{-3.7-E_{p/q}/2}$}{}{}}
\newlabel{sec:S-discussion}{{S43}{165}{The Conclusion in full}{}{}}
\newlabel{sec:S-code}{{S44}{172}{Computational material}{}{}}
\makeatother
